# Supplementary material for: Polariton-induced Purcell effects via a reduced semiclassical electrodynamics approach
Source: arXiv:2412.04694 source file (2025-03-15)
Supplement: Supplementary file 1 [file SI.pdf]

# Supplementary Material

# Polariton-induced Purcell effects via a reduced semiclassical electrodynamics approach

Andres Felipe Bocanegra Vargas[1] and Tao E. Li[1,*]

[1]*Department of Physics and Astronomy,*
*University of Delaware, Newark, Delaware 19716, USA*

## I. ADDITIONAL DATA WHEN $\gamma_{\mathrm{L}} = 4.14 \times 10^{-3}$ eV.

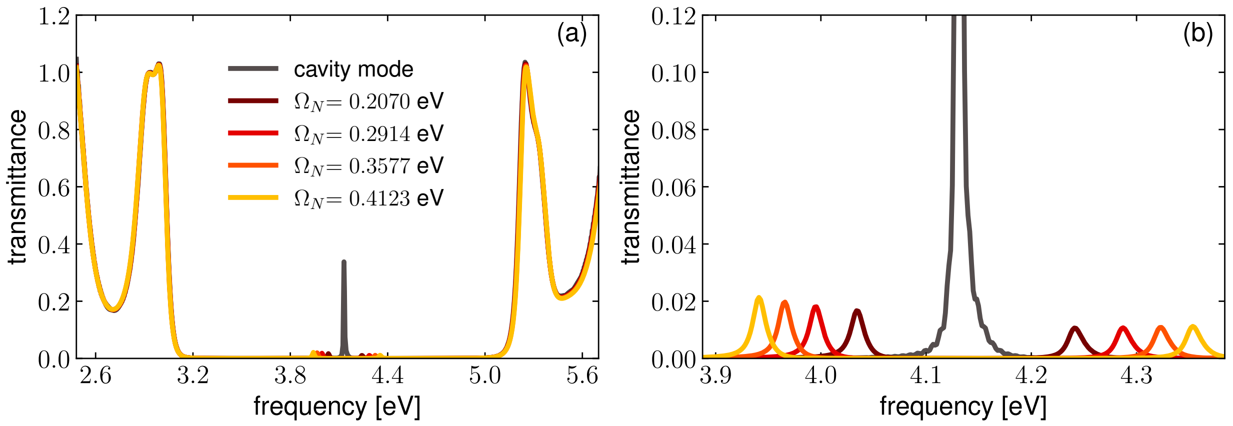


FIG. S1. Linear polariton spectra analogous to Fig. 1b and Fig. 1c except that the dissipation rate of the Lorentz medium is set to $\gamma_{\mathrm{L}} = 4.14 \times 10^{-3}$ eV. Due to the different $\gamma_{\mathrm{L}}$ value used compared to the main text, the corresponding Rabi splitting values are slightly altered and are labeled in part (a).

* taoeli@udel.edu

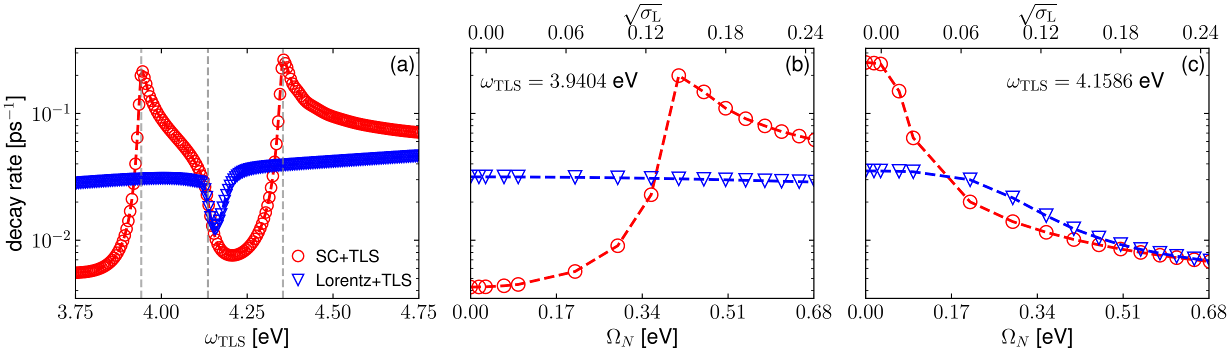


FIG. S2. Parameter dependence of the polariton-induced Purcell effect analogous to Fig. 3 when $\gamma_{\mathrm{L}} = 4.14 \times 10^{-3}$ eV.

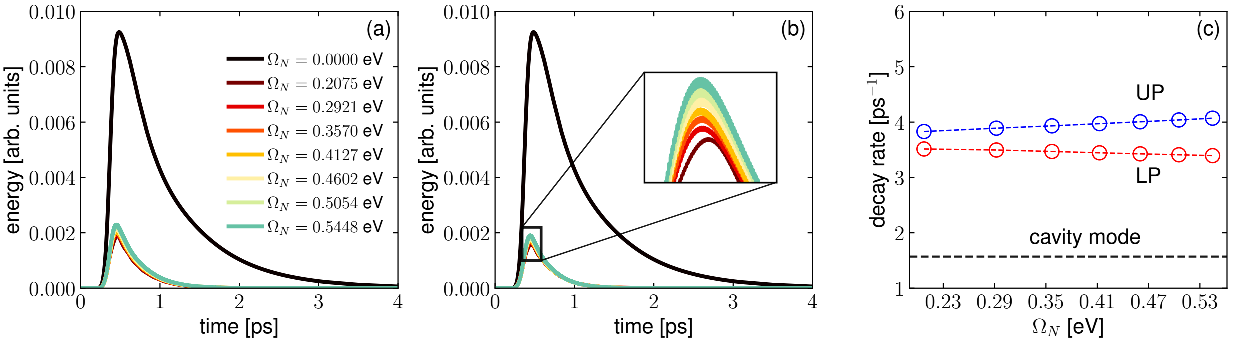


FIG. S3. Simulated polariton energy relaxation dynamics analogous to Fig. 4 when $\gamma_{\mathrm{L}} = 4.14 \times 10^{-3}$ eV.

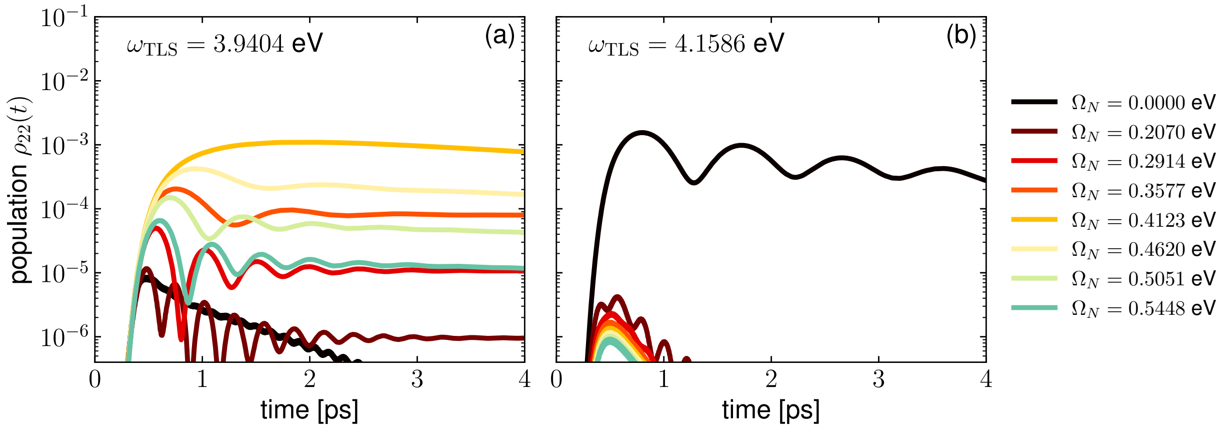


FIG. S4. TLS excited-state population dynamics after the LP excitation analogous to Fig. 5 when $\gamma_{\mathrm{L}} = 4.14 \times 10^{-3}$ eV.

## II. ADDITIONAL DATA WHEN $\gamma_{\rm L} = 4.14 \times 10^{-2}$ eV.

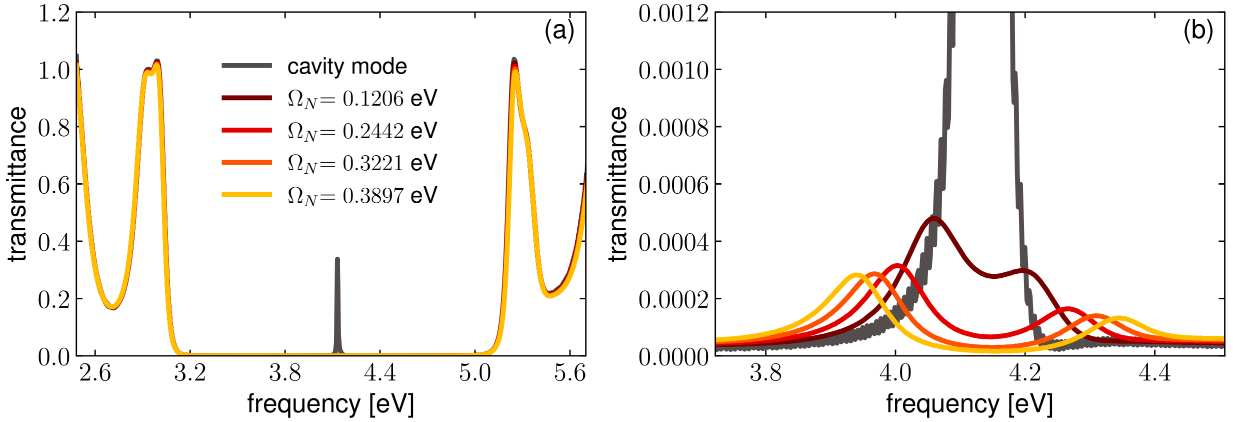


FIG. S5. Linear polariton spectra analogous to Fig. 1b and Fig. 1c except that the dissipation rate of the Lorentz medium is set to $\gamma_{\rm L} = 4.14 \times 10^{-2}$ eV. Due to the significantly larger $\gamma_{\rm L}$ value compared to that in the main text, the corresponding Rabi splitting values are substantially altered and are labeled in part (a).

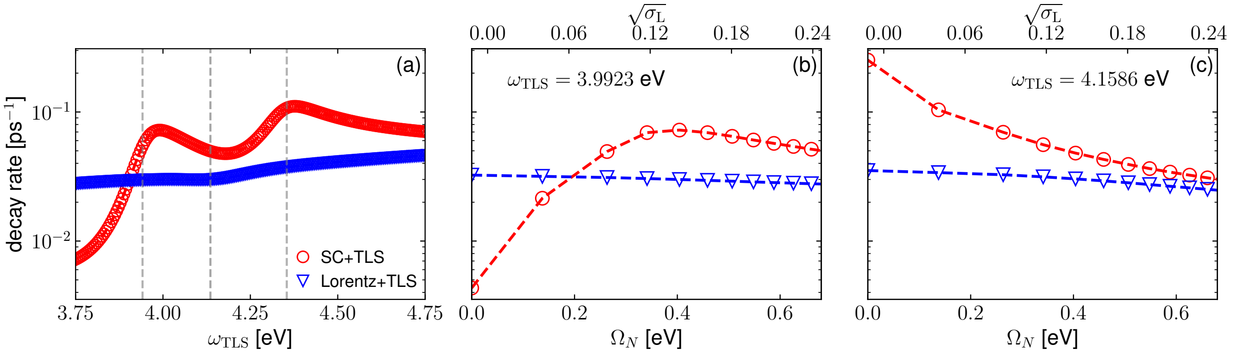


FIG. S6. Parameter dependence of the polariton-induced Purcell effect analogous to Fig. 3 when $\gamma_{\rm L} = 4.14 \times 10^{-2}$ eV. As the Rabi splitting value in part (a) differs significantly from that in the main text, in part (b), the TLS frequency is set to the LP frequency from part (a), corresponding to $\omega_{\rm TLS} = \omega_{\rm LP} = 3.9923$ eV.

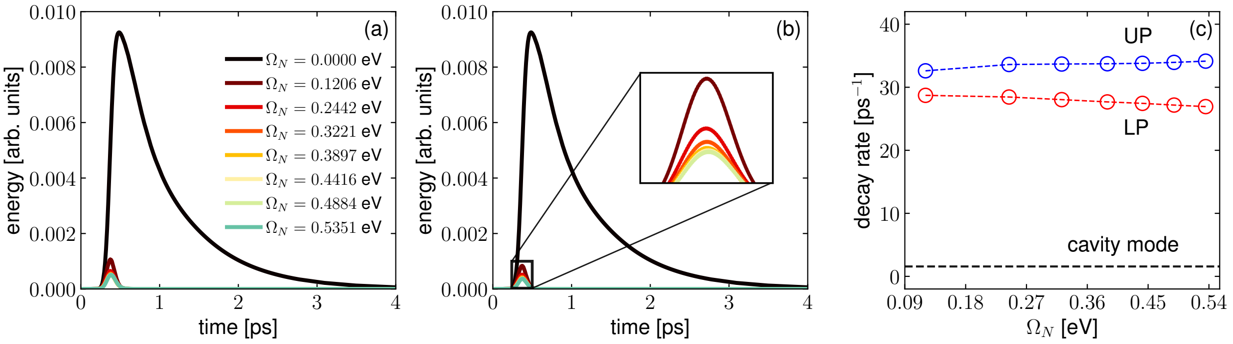


FIG. S7. Simulated polariton energy relaxation dynamics analogous to Fig. 4 when $\gamma_L = 4.14 \times 10^{-2}$ eV.

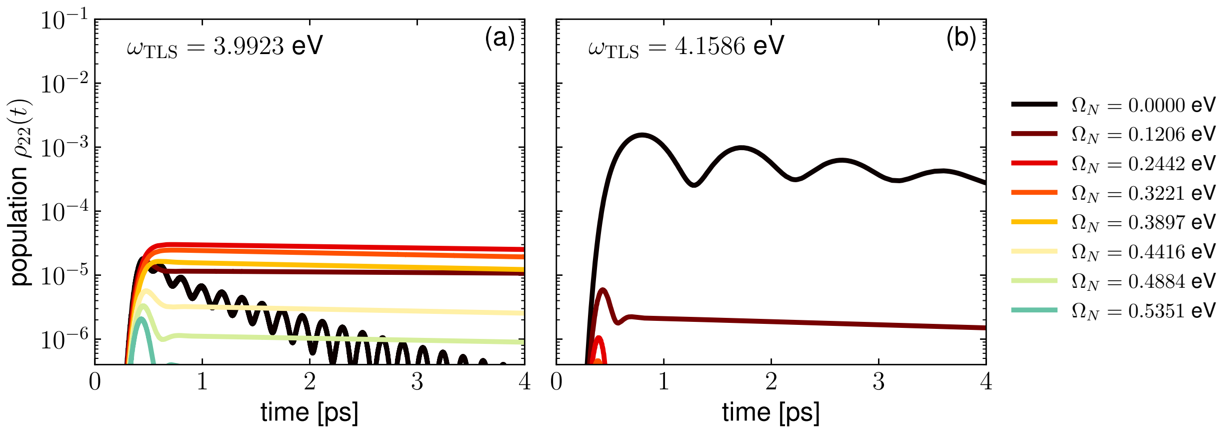


FIG. S8. TLS excited-state population dynamics after the LP excitation analogous to Fig. 5 when $\gamma_L = 4.14 \times 10^{-2}$ eV. As the Rabi splitting value when $\sigma_L = 0.02$ differs significantly from that in the main text, in part (a), the TLS frequency is set to the LP frequency at $\omega_{LP} = 3.9923$ eV.
